# Supplementary material for: Design of secure and robust cognitive system for malware detection
Source: arXiv:2208.02310 source file (2022-08-03)
Supplement: Supplementary file 1 [file Appendix.tex]

%% A sample appendix
%%
%%**********************************************************************
%% Legal Notice:
%% This code is offered as-is without any warranty either
%% expressed or implied; without even the implied warranty of
%% MERCHANTABILITY or FITNESS FOR A PARTICULAR PURPOSE!
%% User assumes all risk.
%% In no event shall any contributor to this code be liable for any damages
%% or losses, including, but not limited to, incidental, consequential, or
%% any other damages, resulting from the use or misuse of any information
%% contained here.
%%**********************************************************************
%%
%% $Id: Appendix.tex,v 1.6 2006/08/25 00:58:50 Owner Exp $
%%

% N.B.: an appendix chapter starts with "appchapter" instead of "chapter"
%
% The first argument in [ ] is the title as displayed in the table of contents
% The second argument is the title as displayed here.  Use \\ as appropriate in
%   this title to get desired line breaks
\appchapter[An Appendix]{An Appendix}

This is an appendix.  Here is a numbered appendix equation:
\begin{equation}
    a^2 + b^2 = c^2.
\end{equation}
